# Supplementary material for: Bridging the Sim2Real Gap: Vision Encoder Pre-Training for Visuomotor Policy Transfer
Source: arXiv:2501.16389 source file (2025-09-07)
Supplement: Supplementary file 1 [file appendix.tex]

% \appendix

% \section*{Appendix}

% \subsection{Code and Data}

% Our code is attached to the supplementary materials. All code and data will be open-sourced upon publication.

\section{Implementation Details}
